# Supplementary material for: Synthesis of layered gold tellurides AuSbTe and Au$_2$Te$_3$ and their semiconducting and metallic behavior
Source: arXiv:2404.16239 ancillary file (2025-02-03)
Supplement: Supplementary file 1 [file Au2Te3_and_AuSbTe_project_2024-04-24_supplement.pdf]

# Synthesis of layered gold tellurides AuSbTe and $Au_2Te_3$ and their semiconducting and metallic behavior

Supplementary Material

Emma A. Pappas, Rong Zhang, Cheng Peng, Robert T. Busch, Jian-Min Zuo, Thomas P. Devereaux, Daniel P. Shoemaker

## Additional Methods

The chemical composition of AuSbTe and $Au_{1.9}Sb_{0.46}Te_{2.64}$ samples was analyzed using a scanning electron microscope (SEM) with energy dispersive x-ray spectroscopy (EDS). Measurements were made on a ThermoFisher Axia ChemiSEM with an accelerating voltage of 20kV and a spot size of 3. The chemical maps of Fig. 1, 2, 8 and 10, were collected over 5 minutes, while the chemical map of Fig. 9 was collected over 1 minute. The color maps of Au (gold), Sb (turquoise) and Te (magenta) are presented to the right of each figure and are laid over a large SEM image of the sample (to the left of each figure). When appropriate, a color map of Ag (green) is also laid over the SEM image to indicate the presence of electrical contacts.

The Van Der Pauw resistivity measurements were carried out in a Quantum Design Physical Property Measurement System DynaCool. Using silver paint and silver epoxy, four gold wire contacts were made on a quarter circle piece of AuSbTe polished to have a uniform thickness of 0.96 mm. The sample was mounted using Kapton tape. The temperature dependent Van Der Pauw measurements shown in Fig. 4 display a very similar shape as the four-point resistivity data collected on AuSbTe (see main text).

# Chemical Vapor Transport Results

Chemical vapor transport (CVT) of a AuSbTe sample with $Sb_2Te_3$, $AuSb_2$, and Au impurities was attempted. A few broken pieces of pellet and $TeCl_4$ powder, which acted as the transport agent, were sealed in an evacuated silica tube. The hot end of the tube was held at 330 °C for 90 h, while the cold end was held at 280 °C. On the hot side, the sample appeared mostly unreacted and only a few water-sensitive transparent crystals (probably chlorides) and a few small tellurium needles were found at the cold end of the tube. Crushing the sample to smaller pieces and increasing the temperatures to 350 °C and 300 °C gave similar results. CVT of a sample containing mostly $AuTe_2$ and $Au_{1.9}Sb_{0.46}Te_{2.64}$ with iodine as the transport agent was also attempted. The reactants placed at the hot end of the tube were held for 90 h at 350 °C and 250 °C. Significant phase separation took place, leaving gold rich phases like Au, $AuTe_2$, and $AuTe_2I$ at the hot end of the tube. The dark product at the cold end of the tube did not look single crystalline and was strongly attached to the silica tube. Neither ends of the tube seemed to contain a single phase and no further attempts at phase identification were made. The poor transport of gold with the iodine halted our CVT efforts for AuSbTe.

# Additional Figures for AuSbTe

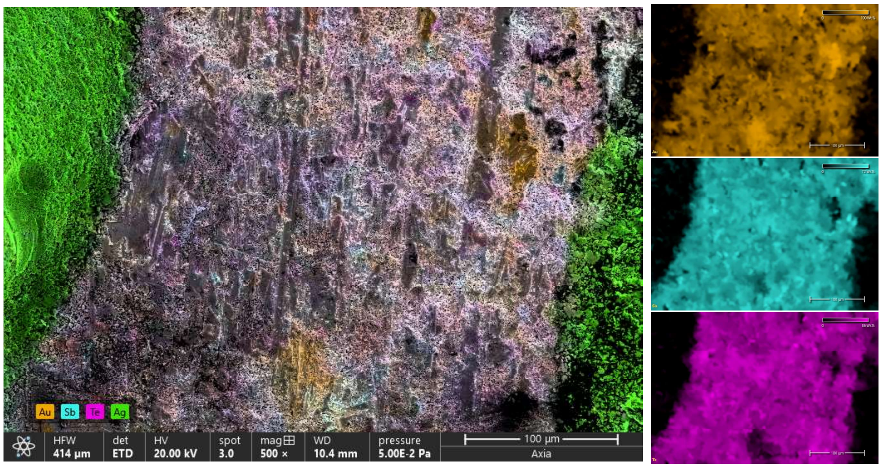


Figure 1: SEM-EDS picture (left) and chemical maps (right) of the AuSbTe sample used for four-point resistivity measurements. The region shown corresponds to the sample surface between the two middle electrical contacts used to measure the voltage drop. These electrical contacts, made with silver paint and epoxy, appear in green on the left and right sides of the main SEM image. The sample was polished into a bar shape for the four-point resistivity measurement, and so its surface shows scratches. The chemical maps of Au (gold), Sb (turquoise) and Te (magenta) show a mostly uniform distribution of the three elements, except for small Au and $Sb_2Te_3$ impurities.

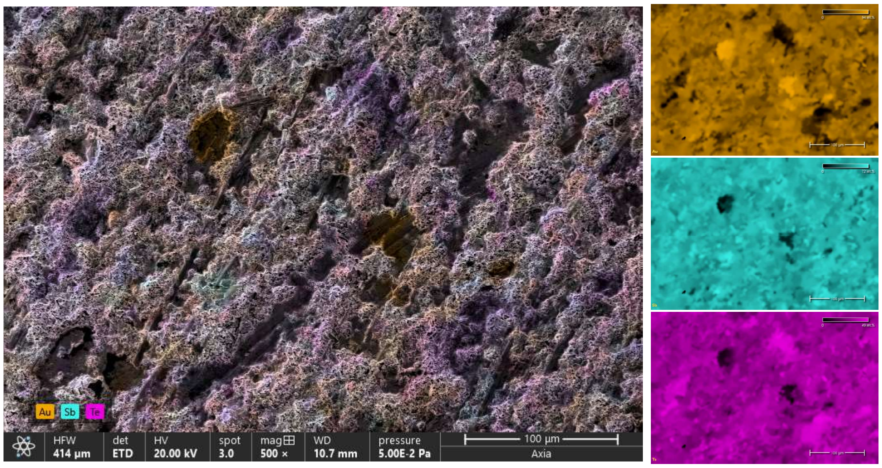


Figure 2: SEM-EDS picture (left) and chemical maps (right) of the AuSbTe sample used for the Van Der Pauw resistivity measurements. A corner piece of the as-synthesized pellet was used, and so only one face had to be polished to obtain a sample with uniform thickness. It is the unpolished face that is shown in this SEM-EDS image. The chemical maps of Au (gold), Sb (turquoise) and Te (magenta) show a mostly uniform distribution of the three elements, except for small Au and $Sb_2Te_3$ impurities.

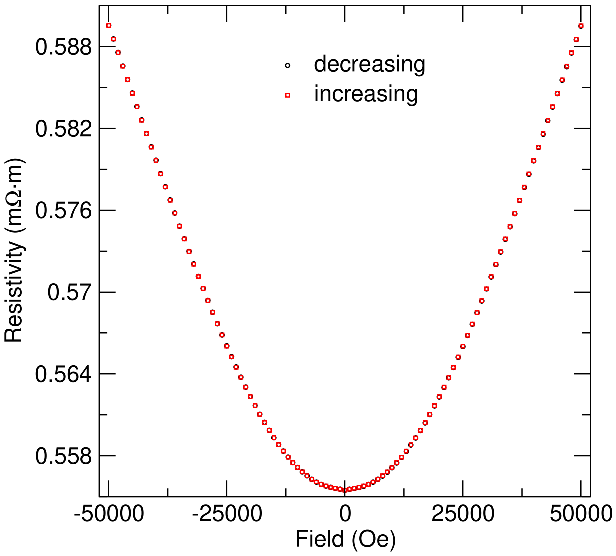


Figure 3: Field dependent four-point resistivity measurement of AuSbTe at 2 K. Black circles and red squares show data collected while decreasing and increasing the magnetic field. The very small change in resistivity across the -5 to 5 T field range indicate that the sample has no significant magnetoresistance.

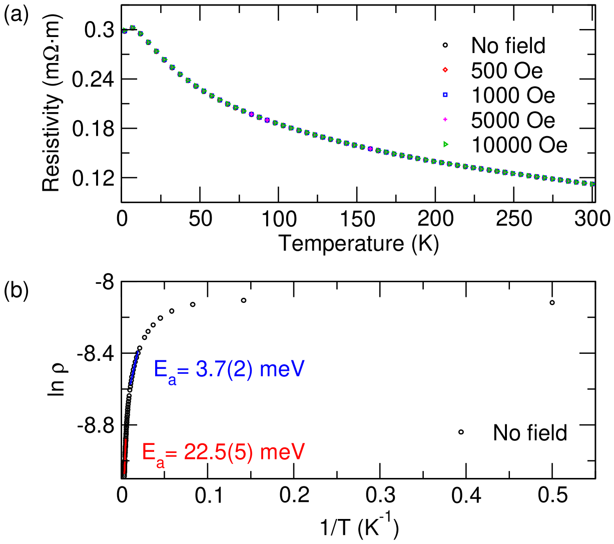


Figure 4: Temperature dependent Van Der Pauw resistivity measurement of AuSbTe. The data is collected on heating. (a) Black circles, red diamond, blue squares, pink pluses and green triangles show data collected without an applied magnetic field, with 500 Oe, 1000 Oe, 5000 Oe and 10000 Oe, respectively. (b) The Arrhenius plot displays a linear behavior only at high temperatures, which is expected considering the metal impurities present in the sample. The activation energy is being fitted for between 50 and 100 K (blue) and between 200 and 300 K (red), with the latter being a better estimate of the value for AuSbTe.

# Additional Figures for $Au_{1.9}Sb_{0.46}Te_{2.64}$

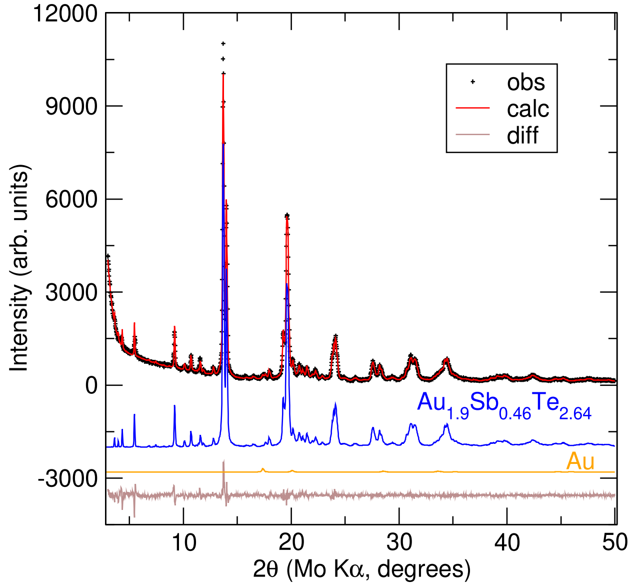


Figure 5: Rietveld refinement of the room temperature PXRD data of the $Au_{1.9}Sb_{0.46}Te_{2.64}$ ingot used for the resistivity measurements. The main phase is fitted to the P$\bar{1}$ structure of $Au_{1.81}Sb_{0.11}Bi_{0.12}Te_{3.04}$ reported by L. Bindi *et al. Can. Mineral.* 56, 129-142 (2018). A minor (6.0(1) wt.%) gold impurity is present in the data.

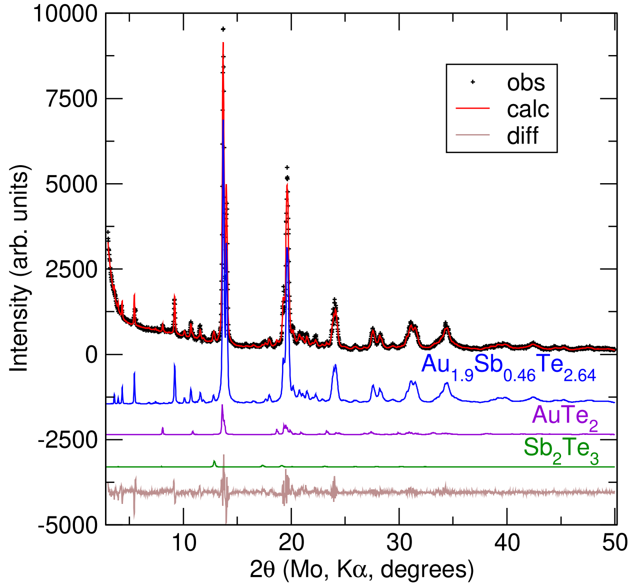


Figure 6: Rietveld refinement of the room temperature PXRD data of the $Au_{1.9}Sb_{0.46}Te_{2.64}$ ingot used for the STEM imaging. The main phase is fitted to the P$\bar{1}$ structure of $Au_{1.81}Sb_{0.11}Bi_{0.12}Te_{3.04}$ reported by L. Bindi *et al. Can. Mineral.* 56, 129-142 (2018). Small $AuTe_2$ (6.5(5) wt.%) and $Sb_2Te_3$ (1.6(3) wt.%) impurities are present.

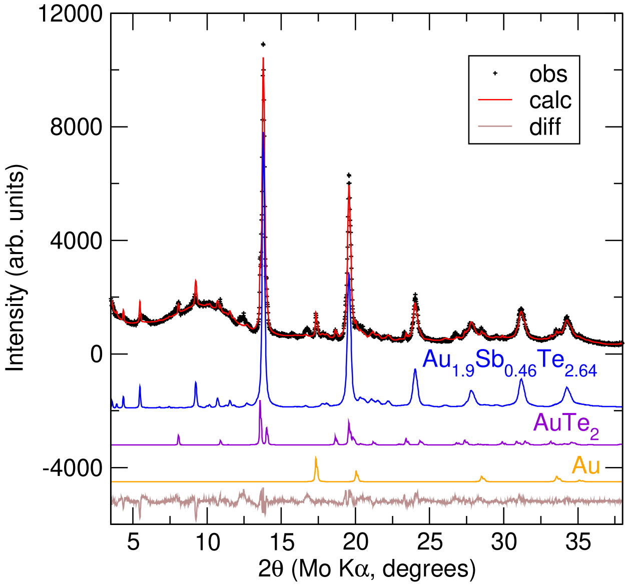


Figure 7: Rietveld refinement of the final room temperature *in situ* PXRD scan of $Au_{1.9}Sb_{0.46}Te_{2.64}$. The main phase is fitted to the P$\bar{1}$ structure of $Au_{1.81}Sb_{0.11}Bi_{0.12}Te_{3.04}$ reported by L. Bindi *et al. Can. Mineral.* 56, 129-142 (2018). Small $AuTe_2$ (10.3(6) wt.%) and Au (3.4(2) wt.%) impurities are present.

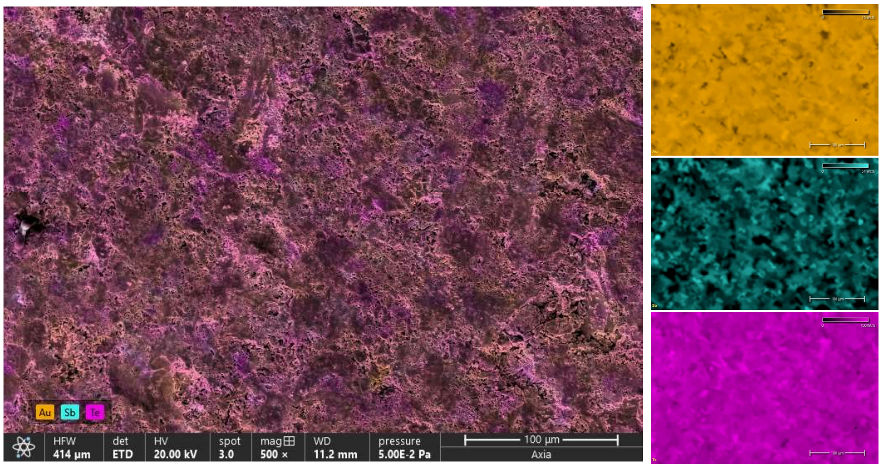


Figure 8: SEM-EDS picture (left) and chemical maps (right) of the $Au_{1.9}Sb_{0.46}Te_{2.64}$ sample used for *in situ* PXRD and DTA measurements. A flat portion of the as-synthesized pellet is shown. The chemical maps of Au (gold), Sb (turquoise) and Te (magenta) show a mostly uniform distribution of the three elements. The Sb chemical map appears a bit less uniform, potentially due to its small proportion in the sample's composition. Upon careful observation, minor Au and Te-rich regions are present.

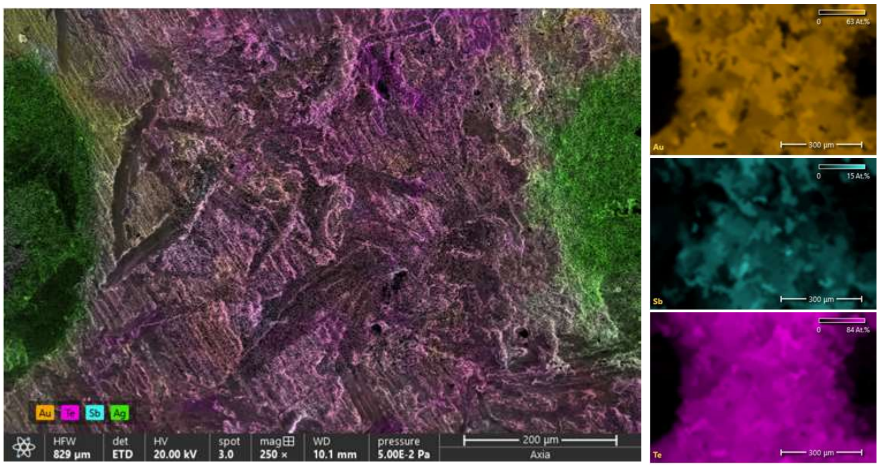


Figure 9: SEM-EDS picture (left) and chemical maps (right) of the $Au_{1.9}Sb_{0.46}Te_{2.64}$ sample used for four-point resistivity measurements. The region shown corresponds to the sample surface between the two middle electrical contacts used to measure the voltage drop. These electrical contacts, made with silver epoxy, appear in green on the left and right sides of the main SEM image. The slow cooled ingot was polished into a bar shape for the four-point resistivity measurement, and so its surface shows scratches. The chemical maps of Au (gold), Sb (turquoise) and Te (magenta) show a mostly uniform distribution of the three elements, except for small Te-rich regions indicating potential $Sb_2Te_3$ impurities. The Sb chemical map appears a bit less uniform, potentially due to its small proportion in the sample's composition.

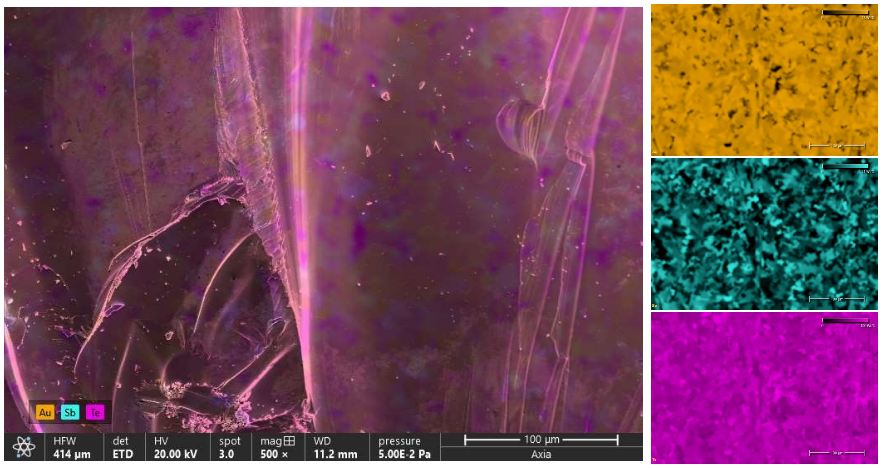


Figure 10: SEM-EDS picture (left) and chemical maps (right) of a portion of the slow cooled $Au_{1.9}Sb_{0.46}Te_{2.64}$ ingot used for STEM imaging. The chemical maps of Au (gold), Sb (turquoise) and Te (magenta) show a mostly uniform distribution of the three elements, except for small Te-rich regions indicating potential $Sb_2Te_3$ impurities. The Sb chemical map appears a bit less uniform, potentially due to its small proportion in the sample's composition.

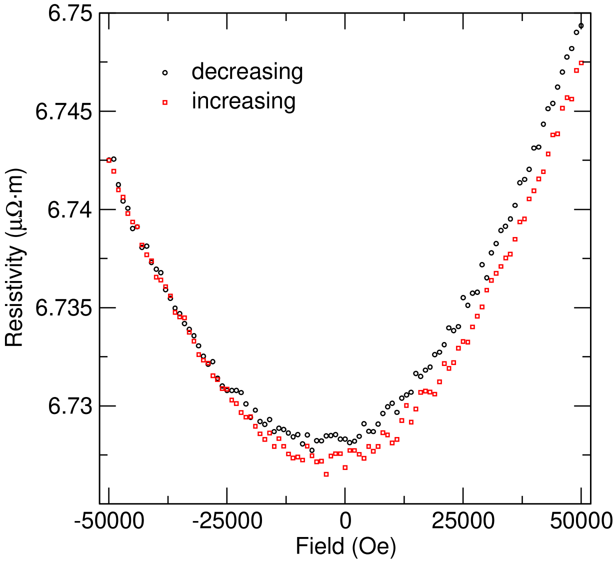


Figure 11: Field dependent four-point resistivity measurement of $Au_{1.9}Sb_{0.46}Te_{2.64}$ at 300 K. Black circles and red squares show data collected while decreasing and increasing the magnetic field. The very small change in resistivity across the -5 to 5 T field range indicate that the sample has no significant magnetoresistance. In light of the extremely small resistivity values, which are associated to more noisy data, the asymmetry of the curve is unimportant. No clear explanation for the asymmetry was identified, but possible causes include low resistance and current, drift, out of equilibrium effects, sample degradation, reaction of the electrical contacts with the sample or experimental artifacts.
